# Supplementary material for: Beyond Words: Advancing Long-Text Image Generation via Multimodal Autoregressive Models
Source: arXiv:2503.20198 source file (2025-03-26)
Supplement: Supplementary file 1 [file supple_data_static_AR.tex]

\begin{table}[h]
    \centering
    \footnotesize
    \begin{tabular}{l|l|l}
    \toprule
        Data Type & Dataset & Sample  \\
        \midrule
        \multirow{2}{*}{Synthetic Data}&Rendered Text Image~\cite{renderedtext} & 0.2M\\
        & ParaGen2M Level 1 & 0.5M\\
        & ParaGen2M Level 2 & 1.5M\\
        &CleanTextSynth~\cite{textatlas5m}&2M\\
        \hline
        \multirow{3}{*}{Natural Image} & LAION-COCO~\cite{laioncoco} & 0.5M \\
        & Marion10M~\cite{textdiffuser} & 3.1M \\
        & AnyWords3M~\cite{anytext} & 0.4M \\
        \midrule
        Total & - & 7.3M\\
        \bottomrule
    \end{tabular}
    \caption{
    \textbf{Statistics of the dataset
    for autoregressive model training}:
    }
    \label{tab:supp_AR_dataset_details}
\end{table}
