# Supplementary material for: Beyond Words: Advancing Long-Text Image Generation via Multimodal Autoregressive Models
Source: arXiv:2503.20198 source file (2025-03-26)
Supplement: Supplementary file 2 [file supple_data_statics.tex]

\begin{table}[h]
    \centering
    \footnotesize
    \begin{tabular}{l|l|l}
    \toprule
        Data Type & Dataset & Sample  \\
        \midrule
        \multirow{4}{*}{OCR Data} & ChartQA~\cite{chartqa} & 0.75M \\
        &DOC-VQA~\cite{docvqa} & 3K\\
        &OCR-VQA~\cite{ocrvqa} & 196K\\
        \hline
        \multirow{2}{*}{Synthetic Data}&Rendered Text Image~\cite{renderedtext} & 7.31M\\
        & ParaGen2M Level 1 & 0.5M\\
        & ParaGen2M Level 2 & 1.5M\\
        \hline
        PDF Document&PDFA~\cite{pdfa_eng_wds}&  1.87M \\
        \hline
        Interlevel Document & IDL-WDS~\cite{pixparse_idl_wds}  & 1.21M \\
        \hline
        Natural Image & COCO-Text~\cite{coco_text} & 112K \\
        \midrule
        Total & - & 13.45M\\
        \bottomrule
    \end{tabular}
    \caption{
    \textbf{Statistics of the  Dataset
    for tokenizer training}:
    }
    \label{tab:supp_8b_dataset_details}
\end{table}
