# Supplementary material for: Beyond Words: Advancing Long-Text Image Generation via Multimodal Autoregressive Models
Source: arXiv:2503.20198 source file (2025-03-26)
Supplement: Supplementary file 3 [file supple_gen_dataset.tex]

\begin{figure*}
    \centering
    \includegraphics[width=\linewidth]{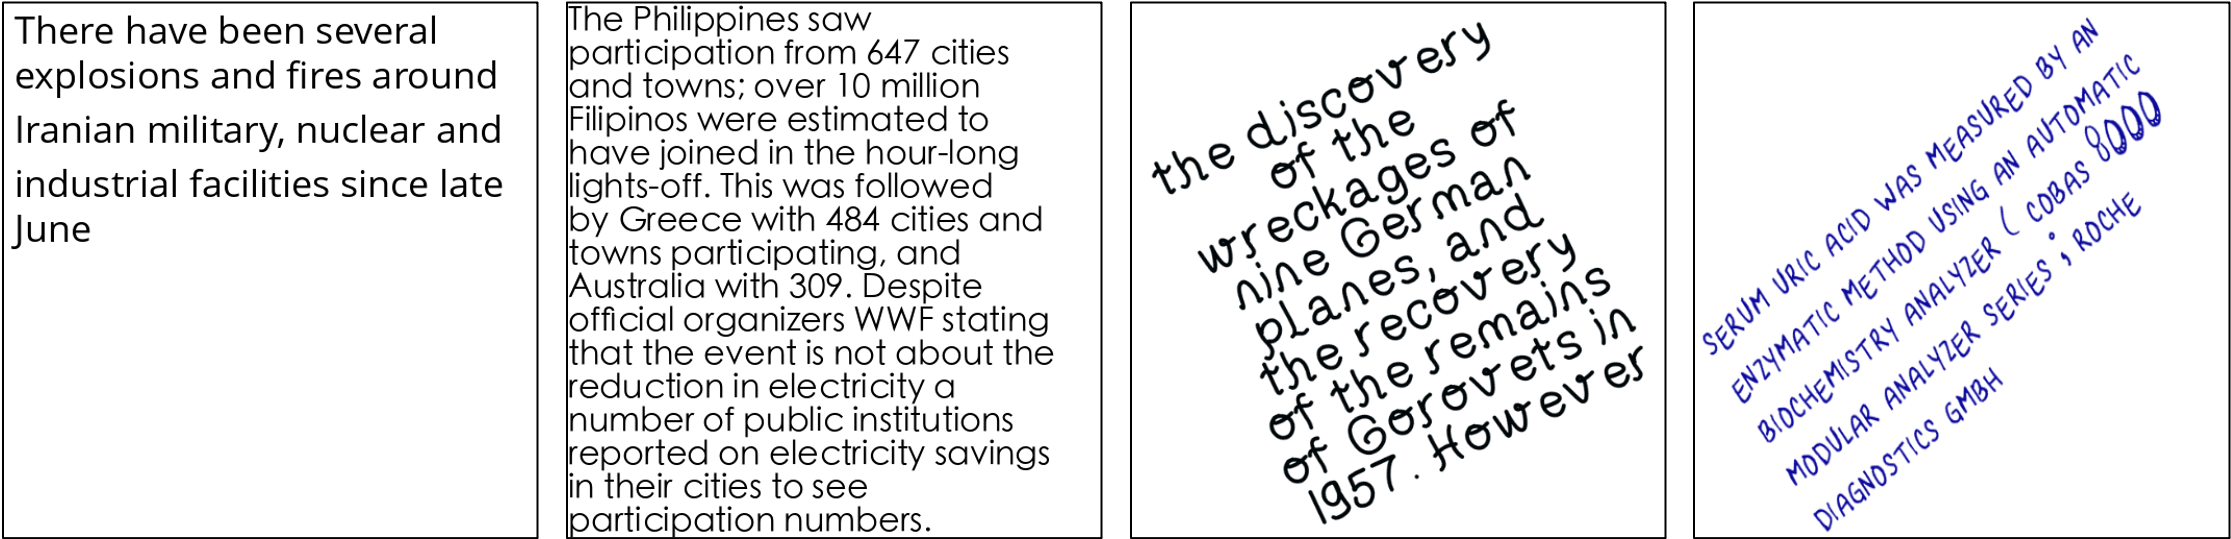}
    \caption{\textbf{Generated a dataset of text renderings with customizable variations.}}
    \label{fig:gen_dataset}
\end{figure*}
